# Supplementary material for: Imitating Graph-Based Planning with Goal-Conditioned Policies
Source: arXiv:2303.11166 source file (2023-03-20)
Supplement: Supplementary file 1 [file 3_additional_comparative.tex]

\begin{figure}[t!]
\begin{minipage}[b]{.45\textwidth}
\centering
\includegraphics[width=1\textwidth]{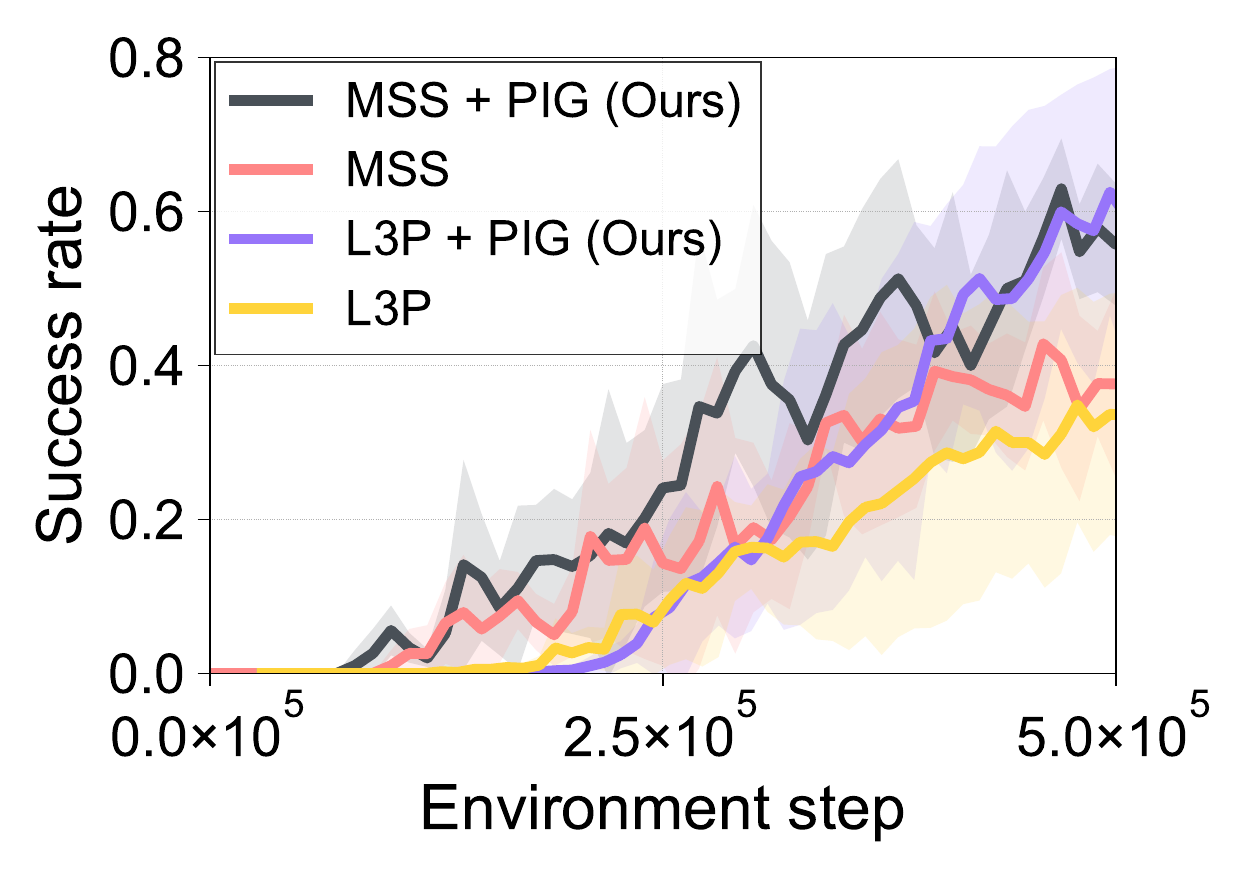}
\caption{This is caption of test1.\newline\newline}
\label{fig:HOG_resolution}
\end{minipage}
\hfill
\begin{minipage}[b]{.45\textwidth}
\centering
\includegraphics[width=1\textwidth]{NeurIPS22/figure/U-shaped AntMaze Planner.pdf}
\caption{Test time success rate of \ALGname and MSS on U-shaped Ant Maze environment. The \textbf{w/o planner} means that planner is not used at test time, so a goal is directly fed into the policy instead of a subgoal. Intriguingly, we find that MSS + \ALGname without a planner can achieve competitive performance to MSS and MSS + \ALGname that utilize a planner.}
\label{fig:planner}
\end{minipage}
\end{figure}
